# Supplementary material for: ViWiD: Leveraging WiFi for Robust and Resource-Efficient SLAM
Source: arXiv:2209.08091 source file (2022-09-16)
Supplement: Supplementary file 1 [file appendix.tex]

% !TEX root = root.tex
\section{APPENDIX}\label{sec:appendix}

To formally define the implementation of iSAM~\cite{gtsam} for \name WiFi SLAM implementaion, let us say that the relative pose measurement provided by the Odometer is $z_i$ with a diagonal covariance matrix $\Sigma_\mathrm{odom} \in \mathbb{R}^{6 \times 6}$. 
This covariance is usually estimated by empirically modeling the noise in the odometer and gyroscope beforehand~\cite{lesson1966simple} which are reported by the manufacturer.
We can then define a state space, $S$, which is a set of robot poses over $N$ time steps in our graph, $S = \{\Vec{p}_i \;|\; \Vec{p}_i = (p^x_i, p^y_i, p^z_i, q^x_i, q^y_i, q^z_i) \in SE(3), \; \forall i \in [1, N]\}$, where each $p_i$ belongs to the Special Euclidean group ($SE(3)$). Specifically, each $\Vec{p}_i$ has two components, the translation in space, $p^t_i = (p^x_i, p^y_i, p^z_i)$, and the quaternion representing its rotation, $p^q_i(q^x_i, q^y_i, q^z_i, 1 - ||(q^x_i, q^y_i, q^z_i)||^2)$.
Next we need to define the measurement model for the odometer factors or the in-between factors between poses $\Vec{p}_i$ and $\Vec{p}_{i+1}$ at two consecutive time steps $\hat{z}^{odom}(\cdot)$. The measurement model can be shown to be:
\begin{align*}
    \hat{z}^{odom}(\Vec{p}_i, \Vec{p}_{i+1}) = \begin{bmatrix} 
                    R(p^q_i)^{-1} (p^t_{i+1} - p^t_{i})^T\\
                    (p^q_{i+1} \ominus p^q_i)_{[1:3]}
                \end{bmatrix} \nonumber 
\end{align*}
where, $R(\cdot) \in SO(3)$ is the rotation matrix corresponding to the given quaternion, $\ominus$ is the relative difference between two quaternions, and $[1:3]$ chooses only the first three elements of the quaternion~\cite{diebel2006representing}. This prediction function now allows us to constrain two consecutive robot poses via a between factor within GraphSLAM \cite{gtsam} and defines an error function between the measurement and prediction as $e_i^{odom}(p_i, p_{i+1}) = z_i^{odom} - \hat{z}_i^{odom}(p_i, p_{i+1})$. 
Similarly, one can define the factor graph for the bearing measurements of AP $j$ at robot position $x_i$ as $\hat{z}^{bot}_{ij}(p_i, x_j) \in \mathbb{R}^2$:
\begin{align}\label{eq:ping-pred}
    &\hat{z}^{bot}_{ij}(p_i, x_j) = \mathrm{Local}(\mathrm{TransformTo}(x_j, p_i), p_i) \\
                                &= \mathrm{Local}([\cos(\phi)\cos(\theta), \cos(\phi)\sin(\theta), \sin(\phi)]^T, p_i) \nonumber
\end{align}
where, $\{p_i \; \forall i \in [1, N]\}\ \bigcup\ \{x_j \; \forall j \in [1, N_{ap}]\}$, for $N$ number of robot poses and $N_{ap}$ WiFi AP poses. Furthermore, \textit{TransformTo}$(\cdot)$ transforms the coordinates of the AP $x_j$ to the coordinate system provided by the robot at $p_i$, in which the AP subtends an elevation angle of $\phi$ and an azimuth angle of $\theta$. \textit{Local}$(\cdot)$ projects this bearing measurement to the tangent plane defined by the current pose of the robot, $p_i$. 
Finally, we also define the covariance of these bearing measurements, $\Sigma_\mathrm{bearing} \in \mathbb{R}^{2 \times 2}$. 

With the factor graph thus constructed, we can define optimization function to find a set of values $S_{opt}$ such that the total error between our predictions, $\hat{z}$'s, and actual measurements, $z$'s, is minimized. 
At a high level, GTSAM framework optimizes for all the variables, $\{p_i \; \forall i \in [1, N]\}\ \bigcup\ \{x_j \; \forall j \in [1, N_{ap}]\}$, end-to-end considering all the measurements, $\{z_i^{odom}$ , $\hat{z}^{AP}_{ij}(p_i, x_j)\} \forall i \in [1, N]$ and $\forall j \in [1, N_{ap}]\}$ together and optimizing for them as a post processing step.

To avoid high compute iSAM is implemented to consider only a part of the nodes.
Specifically, given $I=\{p_i,x_j: i<n,$ $\forall j \in [1, N_{ap}]\}$, where $n$ is the current time instance when a new measurement is added to the factor graph, only a subset of the factors $I_{sub} \subseteq I$ are optimized.
We can estimate the optimized robot poses $S_{opt}^n$ for time instance $n$ by minimizing the total error between our predictions and actual measurements for the subset $I_{sub}$, i.e.
\begin{align}\label{eq:graph-optim-head}
    S_{opt}^n = \argmin_{S} \sum_{i\in I_{sub}} \sum_{j\in I_{sub}}  & \rho\left(\big(e^{bearing}_{ij}\big)^T \Sigma_\mathrm{bearing}^{-1} e^{bearing}_{ij};c\right) \nonumber\\
         & + \sum_{i\in I_{sub}}  \big(e^{odom}_i\big)^T \Sigma_\mathrm{odom}^{-1} e^{odom}_i
\end{align}
where $e^{bearing}_{ij} = z^{bearing}_{ij} - \hat{z}^{bearing}(p_i, x_j)$ is the bearing factor's error between robot and AP poses $i$ and $j$, $\rho$ is the Huber cost function with parameter $c$~\cite{zhang1997parameter}. Thus providing for optimized global robot poses $\{p_i \; \forall i \in I_{sub}\}$ without needing any memory and compute demanding global loop closures.
